# Supplementary material for: Quantum circuit matrix product state ansatz for large-scale simulations of molecules
Source: arXiv:2301.06376 source file (2023-01-16)
Supplement: Supplementary file 2 [file supporting_information.pdf]

# Supporting Information

## Quantum circuit matrix product state ansatz for large-scale simulations of molecules on a quantum computer

Yi Fan,<sup>†</sup> Jie Liu,<sup>‡</sup> Zhenyu Li,<sup>\*,†,‡</sup> and Jinlong Yang<sup>†,‡</sup>

<sup>†</sup>*Hefei National Research Center for Physical Sciences at the Microscale, University of  
Science and Technology of China, Hefei, Anhui 230026, China*

<sup>‡</sup>*Hefei National Laboratory, Hefei, Anhui 230088, China*

E-mail: zyli@ustc.edu.cn

## S1. Potential Energy Curve of H<sub>2</sub>

The potential energy curve of H<sub>2</sub> calculated with bond length R(H-H) from 0.6 to 2.5 Ångstrom is shown in Figure S1. Canonical HF orbitals are used to perform the simulation. QCMPS can converge to chemical accuracy using AU block with  $N_q = 2$  and  $N_l = 1$ . From the bond dimension point of view, the QCMPS ansatz used here is equivalent to a classical MPS with  $D = 2$ .

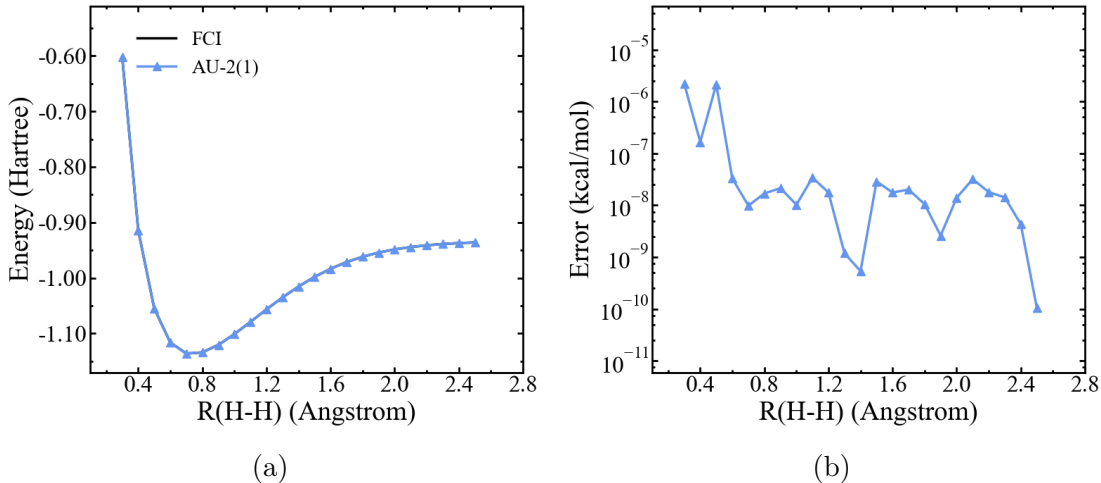

Figure S1: The simulated (a) potential energy curve and (b) error with respect to FCI energy of H<sub>2</sub>, using QCMPS ansatz with AU-2(1) blocks.
